# Supplementary material for: HIVE: HIerarchical Volume Encoding for Neural Implicit Surface Reconstruction
Source: arXiv:2408.01677 source file (2024-08-03)
Supplement: Supplementary file 3 [file vis_supp.tex]

\begin{figure}[h]
\begin{center}

% \begin{subfigure}{0.02\columnwidth}
%     \small{\rotatebox{90}{~~~~~~~~~~~~~~~~~~~~~~~THUman}}
% \end{subfigure}
%
\begin{subfigure}{0.22\columnwidth}
  \centering
  \includegraphics[width=1\columnwidth, trim={3cm 3cm 3cm 2cm}, clip]{figs/compare/thuman/0001/img_210.jpg}
\end{subfigure}
\begin{subfigure}{0.22\columnwidth}
  \centering
  \includegraphics[width=1\columnwidth, trim={11cm 11cm 11cm 5cm}, clip]{figs/compare/thuman/0001/neus_cap_210.jpg}
\end{subfigure}
\begin{subfigure}{0.22\columnwidth}
  \centering
  \includegraphics[width=1\columnwidth, trim={11cm 11cm 11cm 5cm}, clip]{figs/compare/thuman/0001/ours_cap_210.jpg}
\end{subfigure}

% \begin{subfigure}{0.02\columnwidth}
% \small{\rotatebox{90}{~~~~~~~~~~~~~~~~~~~~~~~THUman}}
% \end{subfigure}
%
\begin{subfigure}{0.22\columnwidth}
  \centering
  \includegraphics[width=1\columnwidth, trim={3cm 3cm 3cm 2cm}, clip]{figs/compare/thuman/0212/img_70.jpg}
\end{subfigure}
\begin{subfigure}{0.22\columnwidth}
  \centering
  \includegraphics[width=1\columnwidth, trim={11cm 11cm 11cm 5cm}, clip]{figs/compare/thuman/0212/neus_cap_70.jpg}
\end{subfigure}
\begin{subfigure}{0.22\columnwidth}
  \centering
  \includegraphics[width=1\columnwidth, trim={11cm 11cm 11cm 5cm}, clip]{figs/compare/thuman/0212/ours_cap_70.jpg}
\end{subfigure}

\end{center}
\vspace{-3mm}
 \caption{Visualization comparison of the reconstructed meshes on the THUman-2.0.}
\label{fig:vis_other}
\vspace{-5mm}
\end{figure}
